# Supplementary material for: Scalable Random Feature Latent Variable Models
Source: arXiv:2410.17700 source file (2024-10-23)
Supplement: Supplementary file 1 [file old.tex]

\section{Gaussian Likelihood}

Then the likelihood function can be evaluated 
\begin{align}
    \sum_{m=1}^{M} \log p(\y_m \mid & \X, \W, \ba_m) = \sum_{m=1}^{M}  
    -\frac{N}{2} \log (2 \pi \sigma_{m}^{2}) \nonumber \\ 
    &-\frac{\sigma_m^{-2}}{2} \left( \y_m - \bPhi \ba_m \right)^{\top} \left( \y_m - \bPhi \ba_m \right).
    \label{eq:likelihood}
\end{align}
We first evaluate the expectation of \eqref{eq:likelihood} with respect to $q(\W)$ and $q(\bA)$. For $m$-th term, this evaluation involves assessing the expectations of $\y^{\top}_m \bPhi \ba_m$ and $\ba^{\top}_m \bPhi^{\top} \bPhi \ba_m$ under $q(\W)q(\ba_m)$, i.e., 
\begin{align}
    \mathbb{E}_{q(\W) q(\ba_m)} \left[ \y^{\top}_m \bPhi \ba_m \right] = \y^{\top}_m \mathbb{E}_{q(\W)}[\bPhi ] \mathbb{E}_{q(\ba_m)} [ \ba_m ],
\end{align}
and 
\begin{align}
    & ~~~~\mathbb{E}_{q(\W) q(\ba_m)} \left[ \ba^{\top}_m \bPhi^{\top} \bPhi \ba_m \right] \nonumber \\ 
    &= \operatorname{Tr} \left( \mathbb{E}_{q(\W)} \left[ \bPhi^{\top} \bPhi \right]  \mathbb{E}_{q(\ba_m)} \left[ \ba_m \ba^{\top}_m \right] \right) . 
\end{align}
The values of $\mathbb{E}_{q(\ba_m)} [ \ba_m ]$ and $\mathbb{E}_{q(\ba_m)} \left[ \ba_m \ba^{\top}_m \right]$ can be analytically computed as 
\begin{subequations}
    \begin{align}
    \mathbb{E}_{q(\ba_m)} [ \ba_m ] &= \mathbf{m}_m \\ 
    \mathbb{E}_{q(\ba_m)} \left[ \ba_m \ba^{\top}_m \right] &= \mathbf{S}_m + \mathbf{m}_m \mathbf{m}^{\top}_m . 
    \end{align}
\end{subequations}
Leveraging Identity \ref{identity:1} and employing algebraic operations detailed in Appendix \ref{app:Identity_1}, we can compute:
\begin{align}
    \mathbb{E}_{q(\W)}[\bPhi] = 
    \left[ \begin{array}{ccc}
     \varphi^{\prime}(\x_1), \dots,  
     \varphi^{\prime}(\x_N)
\end{array} \right]^{\top}, 
\label{expectation-phi}
\end{align}
where
\begin{align}
    \varphi^{\prime}(\x_n) &\triangleq \sqrt{\frac{2}{L}}\left[\begin{array}{c}
e^{-\frac{1}{2} \x_n^{\top} \bSigma_1 \x_n} \sin \left(\bmu_{1}^{\top} \x_n\right)  \\
e^{-\frac{1}{2} \x_n^{\top} \bSigma_1 \x_n} \cos \left(\bmu_{1}^{\top} \x_n\right) \\
\vdots \\
e^{-\frac{1}{2} \x_n^{\top} \bSigma_{L/2} \x_n} \sin \left(\bmu_{L/2}^{\top} \x_n \right) \\
e^{-\frac{1}{2} \x_n^{\top} \bSigma_{L/2} \x_n} \cos \left(\bmu_{L/2}^{\top} \x_n \right) 
\end{array}\right]. 
\end{align}
Then, by utilizing Identity \ref{identity:2} and employing algebraic operations detailed in Appendix \ref{app:Identity_2}, we can calculate $\mathbb{E}_{q(\W)} \left[ \bPhi^{\top} \bPhi \right] \in \mathbb{R}^{L \times L}$. Specifically, the value of $\left[\mathbb{E}_{q(\W)} \left[ \bPhi^{\top} \bPhi \right] \right]_{i, j}$ has following several situations, (1) when $i=j$, and $i$ is an odd number, then $\left\{ \mathbb{E}_{q(\mathbf{W})}\left[\boldsymbol{\Phi}^{\top} \boldsymbol{\Phi}\right] \right\}_{i, j}=\sum_{n=1}^{N} \frac{2}{L} \left( \frac{1}{2} + \frac{1}{2} e^{-2 \x_i^{\top} \bSigma_{i \% 2} \x_i \cos(2 \bmu^{\top}_{i \% 2} \x_i) } \right) $; (2) when $i=j$, and $i$ is an even number, then $\left\{ \mathbb{E}_{q(\mathbf{W})}\left[\boldsymbol{\Phi}^{\top} \boldsymbol{\Phi}\right] \right\}_{i, j}=\sum_{n=1}^{N} \frac{2}{L} \left( \frac{1}{2} - \frac{1}{2} e^{-2 \x_i^{\top} \bSigma_{i \% 2} \x_i \cos(2 \bmu^{\top}_{i \% 2} \x_i) } \right) $; (3) when $i \neq j$, and both $i, j$ are even number, then $\left\{ \mathbb{E}_{q(\mathbf{W})}\left[\boldsymbol{\Phi}^{\top} \boldsymbol{\Phi}\right] \right\}_{i, j}=\sum_{n=1}^{N} \frac{2}{L} \sin(\bmu_{i \% 2}^{\top} \x_i) \sin(\bmu_{j \% 2}^{\top} \x_i)   e^{-\frac{1}{2} \x^{\top}_i (\bSigma_{i \% 2} + \bSigma_{j \% 2} ) \x_i }   $; (4) For other situations, when $i$ is an odd number, replace the $\sin$ associated with $i$ in the value defined in situation (3) with $\cos$, and when $j$ is an odd number, replace the $\sin$ associated with $j$ in the value defined in situation (3) with $\cos$.  


\section{Identity 1}
\label{app:Identity_1}
    \begin{identity}
    \begin{align}
        \begin{aligned}
        \mathbb E_{\mathcal{N}(\w ; \bmu, \bSigma)}\left[\cos \left(\w^{\top} \x\right)\right]&=e^{-\frac{1}{2} \x^{\top} \bSigma \x} \cos \left(\bmu^{\top} \x\right),  \\
         \mathbb E_{\mathcal{N}(\w ; \bmu, \bSigma)}\left[\sin \left(\w^{\top} \x\right)\right]&=e^{-\frac{1}{2} \x^{\top} \bSigma \x} \sin \left(\bmu^{\top} \x\right). 
        \end{aligned}
    \end{align}
    \label{identity:1}
    \end{identity}
\begin{proof}
We rely on the characteristic function of the Gaussian distribution to prove this identity.
\begin{align}
    \begin{aligned}
&\mathbb{E}_{\mathcal{N}}(\w ; \bmu, \bSigma)\left[\cos \left(\w^{\top} \x \right)\right] \\
&\quad=\Re\left( E_{\mathcal{N}(\w ; \bmu, \bSigma)}\left[e^{i \w^{\top} \x}\right]\right) \\
&\quad=\Re\left( e^{i \bmu^{\top} \x-\frac{1}{2} \x^{\top} \bSigma \x}\right) \\
&\quad=e^{-\frac{1}{2} \x^{\top} \bSigma \x} \cos \left(\bmu^{\top} \x\right)
\end{aligned}\\
\begin{aligned}
    &\mathbb{E}_{\mathcal{N}}(\w ; \bmu, \bSigma)\left[\sin \left(\w^{\top} \x \right)\right] \\
&\quad=\Im\left( E_{\mathcal{N}(\w ; \bmu, \bSigma)}\left[e^{i \w^{\top} \x}\right]\right) \\
&\quad=\Im\left( e^{i \bmu^{\top} \x-\frac{1}{2} \x^{\top} \bSigma \x}\right) \\
&\quad=e^{-\frac{1}{2} \x^{\top} \bSigma \x} \sin \left(\bmu^{\top} \x\right)
\end{aligned}
\end{align}
where $\Re(\cdot)$ and $\Im(\cdot)$ denote the real part and imaginary part respectively. The transition from the second to the third lines uses the characteristic function of a multivariate Gaussian distribution. 

According to the Identity \ref{identity:1}, the expectation of a single elements for $\sin(\w^{\top}_{l} \x)$ and $\cos(\w^{\top}_{l} \x)$ with respect to $q(\w_{l})$ are
\begin{align}
    \mathbb{E}_{q(\w_{l})} \left[ \cos(\w_{l}^{\top} \x ) \right] = e^{-\frac{1}{2} \x^{\top} \bSigma_{l} \x} \cos \left(\bmu^{\top}_{l} \x\right), \\ 
    \mathbb{E}_{q(\w_{l})} \left[ \sin(\w_{l}^{\top} \x ) \right] = e^{-\frac{1}{2} \x^{\top} \bSigma_{l} \x} \sin \left(\bmu^{\top}_{l} \x\right). 
\end{align}

\end{proof}

\section{Identity 2}
\label{app:Identity_2}
\begin{identity}
    \begin{align}
    \begin{aligned}
    \mathbb E_{\mathcal{N}(\w ; \bmu, \bSigma)}\left[\cos \left(\w^{\top} \x\right)^{2}\right] = \frac{1}{2} +  \frac{1}{2} e^{-2 \x^{\top} \bSigma \x} \cos \left(2 \bmu^{\top} \x\right), \\ 
    \mathbb E_{\mathcal{N}(\w ; \bmu, \bSigma)}\left[\sin \left(\w^{\top} \x\right)^{2}\right] = \frac{1}{2} -\frac{1}{2} e^{-2 \x^{\top} \bSigma \x} \cos \left(2 \bmu^{\top} \x\right).
    \end{aligned}
\end{align}
\label{identity:2}
\end{identity}
\begin{proof}
    Following the identity $\cos (\theta)^{2}=\frac{\cos (2 \theta)+1}{2}, \sin (\theta)^{2}= \frac{1}{2} -\frac{\cos (2 \theta)}{2} $,
\begin{align}
    &\mathbb E_{\mathcal{N}(\w ; \bmu, \bSigma)} \left[ \cos \left(\w^{\top} \x\right)^{2}\right] \nonumber \\
    &=\frac{1}{2} \mathbb E_{\mathcal{N}(\w ; \bmu, \bSigma)} \left[ \cos \left(2 \w^{\top} \x\right)\right]+\frac{1}{2} \nonumber \\ 
    &=\frac{1}{2} e^{-2 \x^{\top} \bSigma \x} \cos \left(2 \bmu^{\top} \x\right)+\frac{1}{2}
\end{align}
\begin{align}
    &\mathbb E_{\mathcal{N}(\w ; \bmu, \bSigma)} \left[ \sin \left(\w^{\top} \x\right)^{2}\right] \nonumber \\
    &=\frac{1}{2} - \frac{1}{2} \mathbb E_{\mathcal{N}(\w ; \bmu, \bSigma)} \left[ \cos \left(2 \w^{\top} \x\right)\right] \nonumber \\ 
    &=\frac{1}{2} -  \frac{1}{2} e^{-2 \x^{\top} \bSigma \x} \cos \left(2 \bmu^{\top} \x\right)
\end{align}
\end{proof}
Building upon this identity, we could evaluate $\mathbb{E}_{q(\W)} \left[ \bPhi^{\top} \bPhi \right]$, an $L \times L$ matrix, where
\begin{align}
    & \left(\mathbb E_{q(\W)}\left[  \bPhi^{\top} \bPhi \right] \right)_{i, j} = \nonumber \\ 
        & \left\{  
             \begin{array}{c}  
             \sum_{n=1}^{N} \frac{2}{L} \mathbb E_{q\left(\w_{i},  \w_{j} \right)}\left[\cos \left(\w_{i}^{\top} \x_{n}\right)\right. \left.\cdot \cos \left(\w_{j}^{\top} \x_{n}\right)\right] \\
             ~~ \text{where~~} i, j \in \mathbb{R}^{2k}  \\
             \sum_{n=1}^{N} \frac{2}{L} \mathbb E_{q\left(\w_{i}, \w_{j} \right)}\left[\cos \left(\w_{i}^{\top} \x_{n}\right)\right. \left.\cdot \sin \left(\w_{j}^{\top} \x_{n}\right)\right]
              \\ 
              ~~\text{where~~} i \in \mathbb{R}^{2k}, j \in \mathbb{R}^{2k+1} \\ 
            \sum_{n=1}^{N} \frac{2}{L} \mathbb E_{q\left(\w_{i}, \w_{j} \right)}\left[\sin \left(\w_{i}^{\top} \x_{n}\right)\right. \left.\cdot \cos \left(\w_{j}^{\top} \x_{n}\right)\right]
              \\ 
              ~~\text{where~~} i \in \mathbb{R}^{2k+1}, j \in \mathbb{R}^{2k} \\ 
             \sum_{n=1}^{N} \frac{2}{L} \mathbb E_{q\left(\w_{i}, \w_{j} \right)}\left[\sin \left(\w_{i}^{\top} \x_{n}\right)\right. \left.\cdot \sin \left(\w_{j}^{\top} \x_{n}\right)\right] \\
             ~~\text{where~~} i, j \in \mathbb{R}^{2k+1}
             \end{array}  
\right. ,
\label{eq:expexp_phi}
\end{align}
for $i, j \leq L/2$. Moreover, for $i \neq j$, through independence we could break the expectation of each term into
\begin{align}
    \left\{  
             \begin{array}{c}  
              \sum_{n=1}^{N} \frac{2}{L} \mathbb E_{q(\w_i)} \left[ \cos \left(\w_{i}^{\top}  \x_{i}\right) \right] \cdot
             \mathbb E_{q(\w_j)} \left[ \cos \left(\w_{j}^{\top}  \x_{i}\right) \right]\\
              ~~ \text{where~~} i, j \in \mathbb{R}^{2k},  \\
              \sum_{n=1}^{N} \frac{2}{L} \mathbb E_{q(\w_i)} \left[ \cos \left(\w_{i}^{\top}  \x_{i}\right) \right] \cdot
             \mathbb E_{q(\w_j)} \left[ \sin \left(\w_{j}^{\top}  \x_{i}\right) \right]\\
              ~~\text{where~~} i \in \mathbb{R}^{2k}, j \in \mathbb{R}^{2k+1}, \\ 
            \sum_{n=1}^{N} \frac{2}{L} \mathbb E_{q(\w_i)} \left[ \sin \left(\w_{i}^{\top}  \x_{i}\right) \right] \cdot
             \mathbb E_{q(\w_j)} \left[ \cos \left(\w_{j}^{\top}  \x_{i}\right) \right]\\
              ~~\text{where~~} i \in \mathbb{R}^{2k+1}, j \in \mathbb{R}^{2k}, \\ 
              \sum_{n=1}^{N} \frac{2}{L} \mathbb E_{q(\w_i)} \left[ \sin \left(\w_{i}^{\top}  \x_{i}\right) \right] \cdot
             \mathbb E_{q(\w_j)} \left[ \sin \left(\w_{j}^{\top}  \x_{i}\right) \right] \\
             ~~\text{where~~} i, j \in \mathbb{R}^{2k+1},
             \end{array}  
\right. 
\end{align}
and for $i=j$, 
\begin{align}
\left\{
\begin{array}{c}
      \sum_{n=1}^{N} \frac{2}{L} \mathbb E_{q\left(\w_{i}\right)} \left[ \cos \left(\w_{i}^{\top} \x_i \right)^{2}\right]
     ~~\text{where}~~ i \in \mathbb{R}^{2k},
      \\
      \sum_{n=1}^{N} \frac{2}{L} \mathbb E_{q\left(\w_{i}\right)} \left[ \sin \left(\w_{i}^{\top} \x_i \right)^{2}\right]
      ~~\text{where}~~ i \in \mathbb{R}^{2k+1}. 
\end{array}
\right.
\end{align}
The computation of the expectation for the matrix element where $i \neq j$ is facilitated by employing Identity \ref{identity:1} as demonstrated in Appendix \ref{app:Identity_1}. Meanwhile, for the element where $i=j$, the procedure can be guided by the instructions provided in Identity \ref{identity:2}.

% \section{Inference $\z$}

% \begin{align}
%     &\mathbb{E}_{\W}\left[ \log p\left(\W \mid \z \right)\right]  \\
%     &=
%     \sum_{l=1}^{L/2} \sum_{k=1}^{K} \mathbb E_{\w_l} \left[ \log \mathcal{N}_{Q}(\bmu_{z_l}, \bSigma_{z_l})^{\mathbf{1}\left[z_l=k\right]} \right] \nonumber \\ 
%     &= \sum_{l=1}^{L/2} \sum_{k=1}^{K} \mathbb E_{\w_l} \left[ p(z_l = k) \log \mathcal{N}_{Q}(\bmu_{k}, \bSigma_{k}) \right]  \nonumber \\ 
%     &= \sum_{l=1}^{L/2} \sum_{k=1}^{K} \mathbb E_{\w_l} \Bigg[ p(z_l = k) \Big\{ \log (2\pi)^{-\frac{Q}{2}} |\bSigma_k|^{-1/2} \nonumber\\
%     &~~~- \frac{1}{2}\left( (\w-\bmu_k)^{\top} \bSigma_{k}^{-1} (\w - \bmu_k)\right)   \Big\} \Bigg] \nonumber  \\
%     &= \sum_{l=1}^{L/2} \sum_{k=1}^{K} p(z_l = k) \Bigg[   \log (2\pi)^{-\frac{Q}{2}} |\bSigma_k|^{-1/2} \nonumber\\
%     &~~~- \frac{1}{2} \mathbb{E}_{\w} \left( \w^{\top} \bSigma_{k}^{-1} \w - 2 \w^{\top} \bSigma_{k}^{-1}\bmu_{k} + \bmu_{k}^{\top} \bSigma_{k}^{-1} \bmu_{k}  \right)    \Bigg] \nonumber  \\ 
%     &= \sum_{l=1}^{L/2} \sum_{k=1}^{K} p(z_l = k) \Bigg[   \log (2\pi)^{-\frac{Q}{2}} |\bSigma_k|^{-1/2} \nonumber\\
%     &~~~- \frac{1}{2} \left( \bmu^{\top}_{l} \bSigma_{k}^{-1} \bmu_{l} + \operatorname{Tr}(\bSigma^{-1}_k \bSigma_{l}) - 2 \bmu^{\top}_{l} \bSigma_{k}^{-1}\bmu_{k} + \bmu_{k}^{\top} \bSigma_{k}^{-1} \bmu_{k}  \right)    \Bigg] \nonumber  \\ 
%     &= \sum_{l=1}^{L/2} \sum_{k=1}^{K} p(z_l = k) \Bigg[   \log (2\pi)^{-\frac{Q}{2}} |\bSigma_k|^{-1/2} +  \bmu^{\top}_{l} \bSigma_{k}^{-1}\bmu_{k}  \nonumber\\
%     &~~~- \frac{1}{2} \left( \bmu^{\top}_{l} \bSigma_{k}^{-1} \bmu_{l} + \operatorname{Tr}(\bSigma^{-1}_k \bSigma_{l}) + \bmu_{k}^{\top} \bSigma_{k}^{-1} \bmu_{k}  \right)    \Bigg] \nonumber  
% \end{align}

% \section{Experiments}
% \label{app:dataset}
